# Supplementary material for: SutraNets: Sub-series Autoregressive Networks for Long-Sequence, Probabilistic Forecasting
Source: arXiv:2312.14880 source file (2023-12-22)
Supplement: Supplementary file 1 [file all_forecasts_fig.tex]

\begin{figure}
  \centering {\makebox[\textwidth][c]{
      \begin{subfigure}{\shrinkfigthreeb\textwidth}
        \begin{tikzpicture}
          \node (img1) {\includegraphics[width=\textwidth]{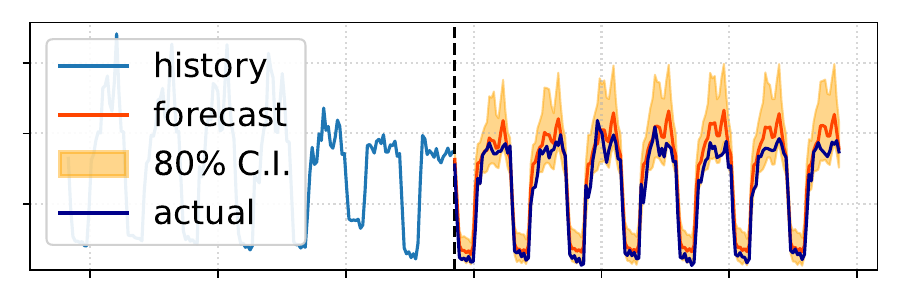}};
          \node[above of=img1, draw=none, align=center, fill=white, yshift=0.0cm, xshift=0.0cm, node distance=0.96cm, anchor=center] {\scriptsize \textbf{$\backfillprevs$}};
        \end{tikzpicture}
      \end{subfigure}
      \hspace{-2mm}
      \begin{subfigure}{\shrinkfigthreeb\textwidth}
        \begin{tikzpicture}
          \node (img1) {\includegraphics[width=\textwidth]{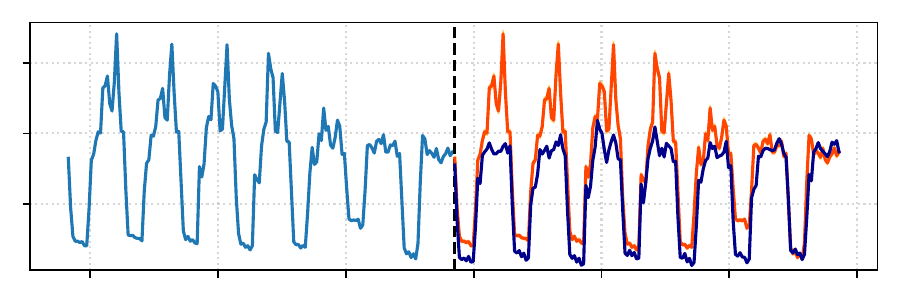}};
          \node[above of=img1, draw=none, align=center, fill=white, yshift=0.0cm, xshift=0.0cm, node distance=0.96cm, anchor=center] {\scriptsize \textbf{$\seasonalnaivew$}};
        \end{tikzpicture}
      \end{subfigure}
      \hspace{-2mm}
      \begin{subfigure}{\shrinkfigthreeb\textwidth}
        \begin{tikzpicture}
          \node (img1) {\includegraphics[width=\textwidth]{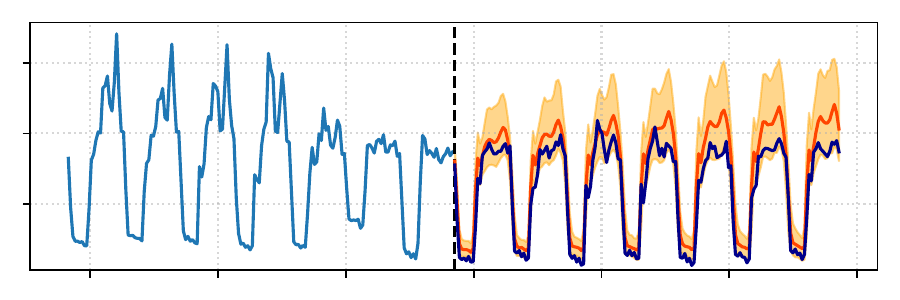}};
          \node[above of=img1, draw=none, align=center, fill=white, yshift=0.0cm, xshift=0.0cm, node distance=0.96cm, anchor=center] {\scriptsize \textbf{$\ctofar$}};
        \end{tikzpicture}
      \end{subfigure}
  }}
  \mbox{}
  \vspace{-3mm}
  \mbox{}
  \centering {\makebox[\textwidth][c]{
      \begin{subfigure}{\shrinkfigthreeb\textwidth}
        \begin{tikzpicture}
          \node (img1) {\includegraphics[width=\textwidth]{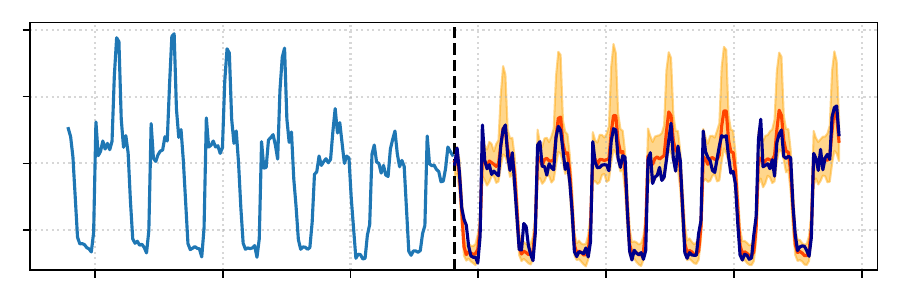}};
        \end{tikzpicture}
      \end{subfigure}
      \hspace{-2mm}
      \begin{subfigure}{\shrinkfigthreeb\textwidth}
        \begin{tikzpicture}
          \node (img1) {\includegraphics[width=\textwidth]{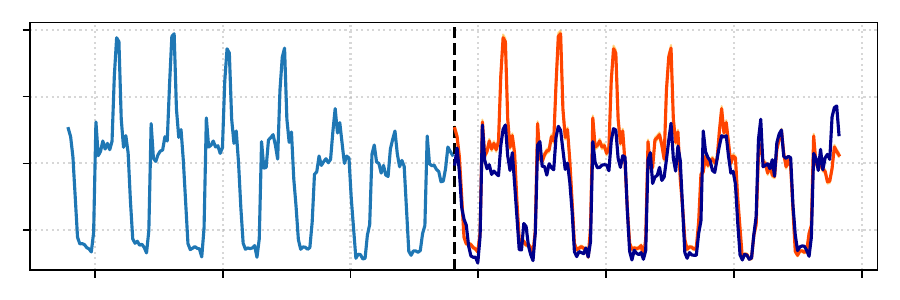}};
        \end{tikzpicture}
      \end{subfigure}
      \hspace{-2mm}
      \begin{subfigure}{\shrinkfigthreeb\textwidth}
        \begin{tikzpicture}
          \node (img1) {\includegraphics[width=\textwidth]{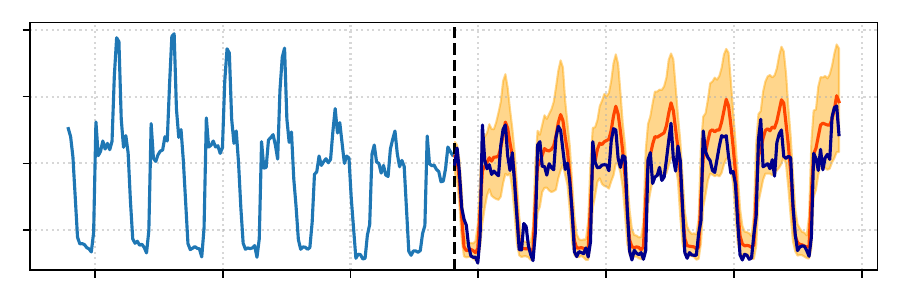}};
        \end{tikzpicture}
      \end{subfigure}
  }}
  \mbox{}
  \vspace{-3mm}
  \mbox{}
  \centering {\makebox[\textwidth][c]{
      \begin{subfigure}{\shrinkfigthreeb\textwidth}
        \begin{tikzpicture}
          \node (img1) {\includegraphics[width=\textwidth]{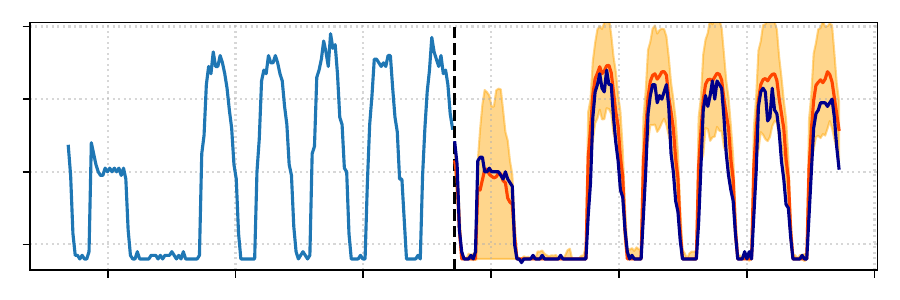}};
        \end{tikzpicture}
      \end{subfigure}
      \hspace{-2mm}
      \begin{subfigure}{\shrinkfigthreeb\textwidth}
        \begin{tikzpicture}
          \node (img1) {\includegraphics[width=\textwidth]{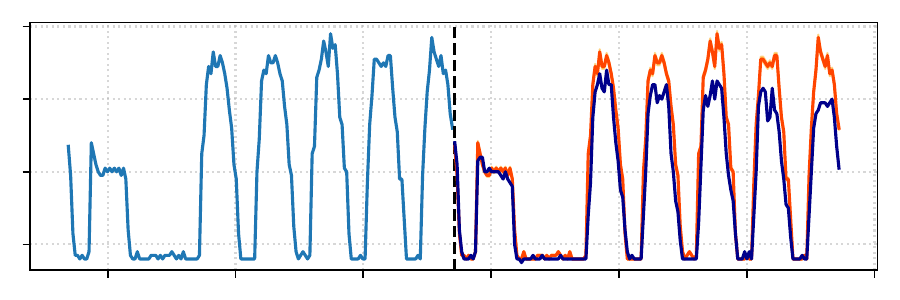}};
        \end{tikzpicture}
      \end{subfigure}
      \hspace{-2mm}
      \begin{subfigure}{\shrinkfigthreeb\textwidth}
        \begin{tikzpicture}
          \node (img1) {\includegraphics[width=\textwidth]{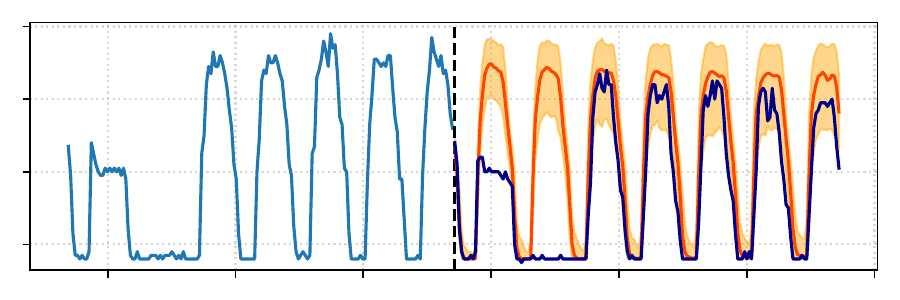}};
        \end{tikzpicture}
      \end{subfigure}
  }}
  \mbox{}
  \vspace{-3mm}
  \mbox{}
  \centering {\makebox[\textwidth][c]{
      \begin{subfigure}{\shrinkfigthreeb\textwidth}
        \begin{tikzpicture}
          \node (img1) {\includegraphics[width=\textwidth]{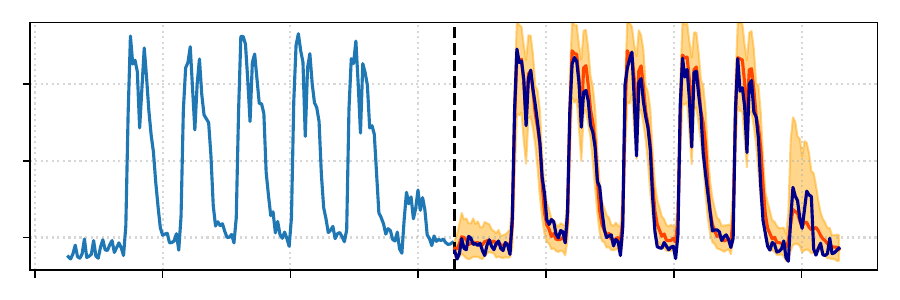}};
        \end{tikzpicture}
      \end{subfigure}
      \hspace{-2mm}
      \begin{subfigure}{\shrinkfigthreeb\textwidth}
        \begin{tikzpicture}
          \node (img1) {\includegraphics[width=\textwidth]{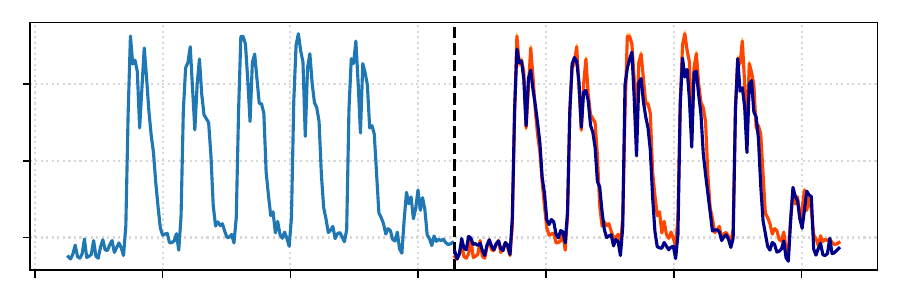}};
        \end{tikzpicture}
      \end{subfigure}
      \hspace{-2mm}
      \begin{subfigure}{\shrinkfigthreeb\textwidth}
        \begin{tikzpicture}
          \node (img1) {\includegraphics[width=\textwidth]{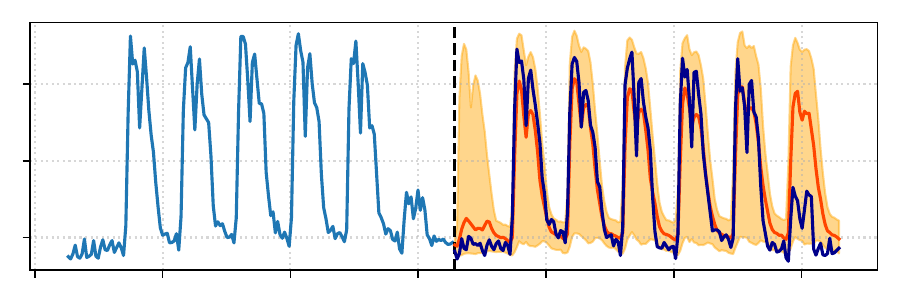}};
        \end{tikzpicture}
      \end{subfigure}
  }}
  \caption{Forecasts and 80\% intervals for $\elec$ series.
    $\backfillprevs$ performs well with a changepoint (rows 1 \& 2,
    where $\seasonalnaive$ fails) and with weekly seasonality (rows 3 \&
    4, where $\ctofar$ fails).\label{fig:forecasts}}
\end{figure}
